# Supplementary material for: Exploring the Meaningfulness of Nearest Neighbor Search in High-Dimensional Space
Source: arXiv:2410.05752 source file (2024-10-08)
Supplement: Supplementary file 1 [file appendix_main.tex]

\newpage

\appendix

\section{Appendix Overview}

In the appendix section of the paper, we conduct extensive study on the following topics:
\begin{enumerate}
    \item How do different generation method for high-dimensional vector could impact the meaningfulness of the Nearest Neighbor Search, given the same source dataset and dimensionality. In this experiment, we discuss both of the image data and the text data.
    \item We provide an overview on how various embeddings models might impact the meaningfulness of the Nearest Neighbor search ? 
\end{enumerate}

Additionally, we propose brief discussion on some technical details of the experiments. 

\section{Generation Method of High-Dimensional Vector}

In this section of the experiment, we include experiment results on how different generation method could impact the meaningfulness of the Nearest Neighbor search problem, for text and image data, in terms of the Relative Contrast. Specifically, for both of text and image data, there are more than one approach in generating the high-dimensional vector as its structured representation. Thus, it will be necessary for us to further investigate into the properties and features of those different vectors. Also, to ensure the comprehensiveness, we also include statistics on the most prestigious datasets for ANN search: SIFT1M\cite{sift} and GIST1M\cite{gist}. 

\subsection{Image Data}

Firstly, let's investigate deeper into the case when the image is the source data. And the generation method of the image could be divided into two categories: Image Feature Extraction and Image Embedding. Specifically, image feature extraction is achieved by Convolution Neural Network (CNN), where the output of the last convolution layer is extracted and considered as the feature vector; and the image embedding is computed by the State-of-the-Art CLIP\cite{CLIP} model. And the dimensionality of all image vector in this section is $512$, which is a common dimensionality for image based models.

Specifically, the Convolution Neural Network involved in the experiment are: ResNet18\cite{resnet}, ResNet34\cite{resnet}, SqueezeNet\cite{squeezenet}, and VGG16\cite{vgg}.

\begin{figure}[htp]
    \centering
    \includegraphics[width=\textwidth]{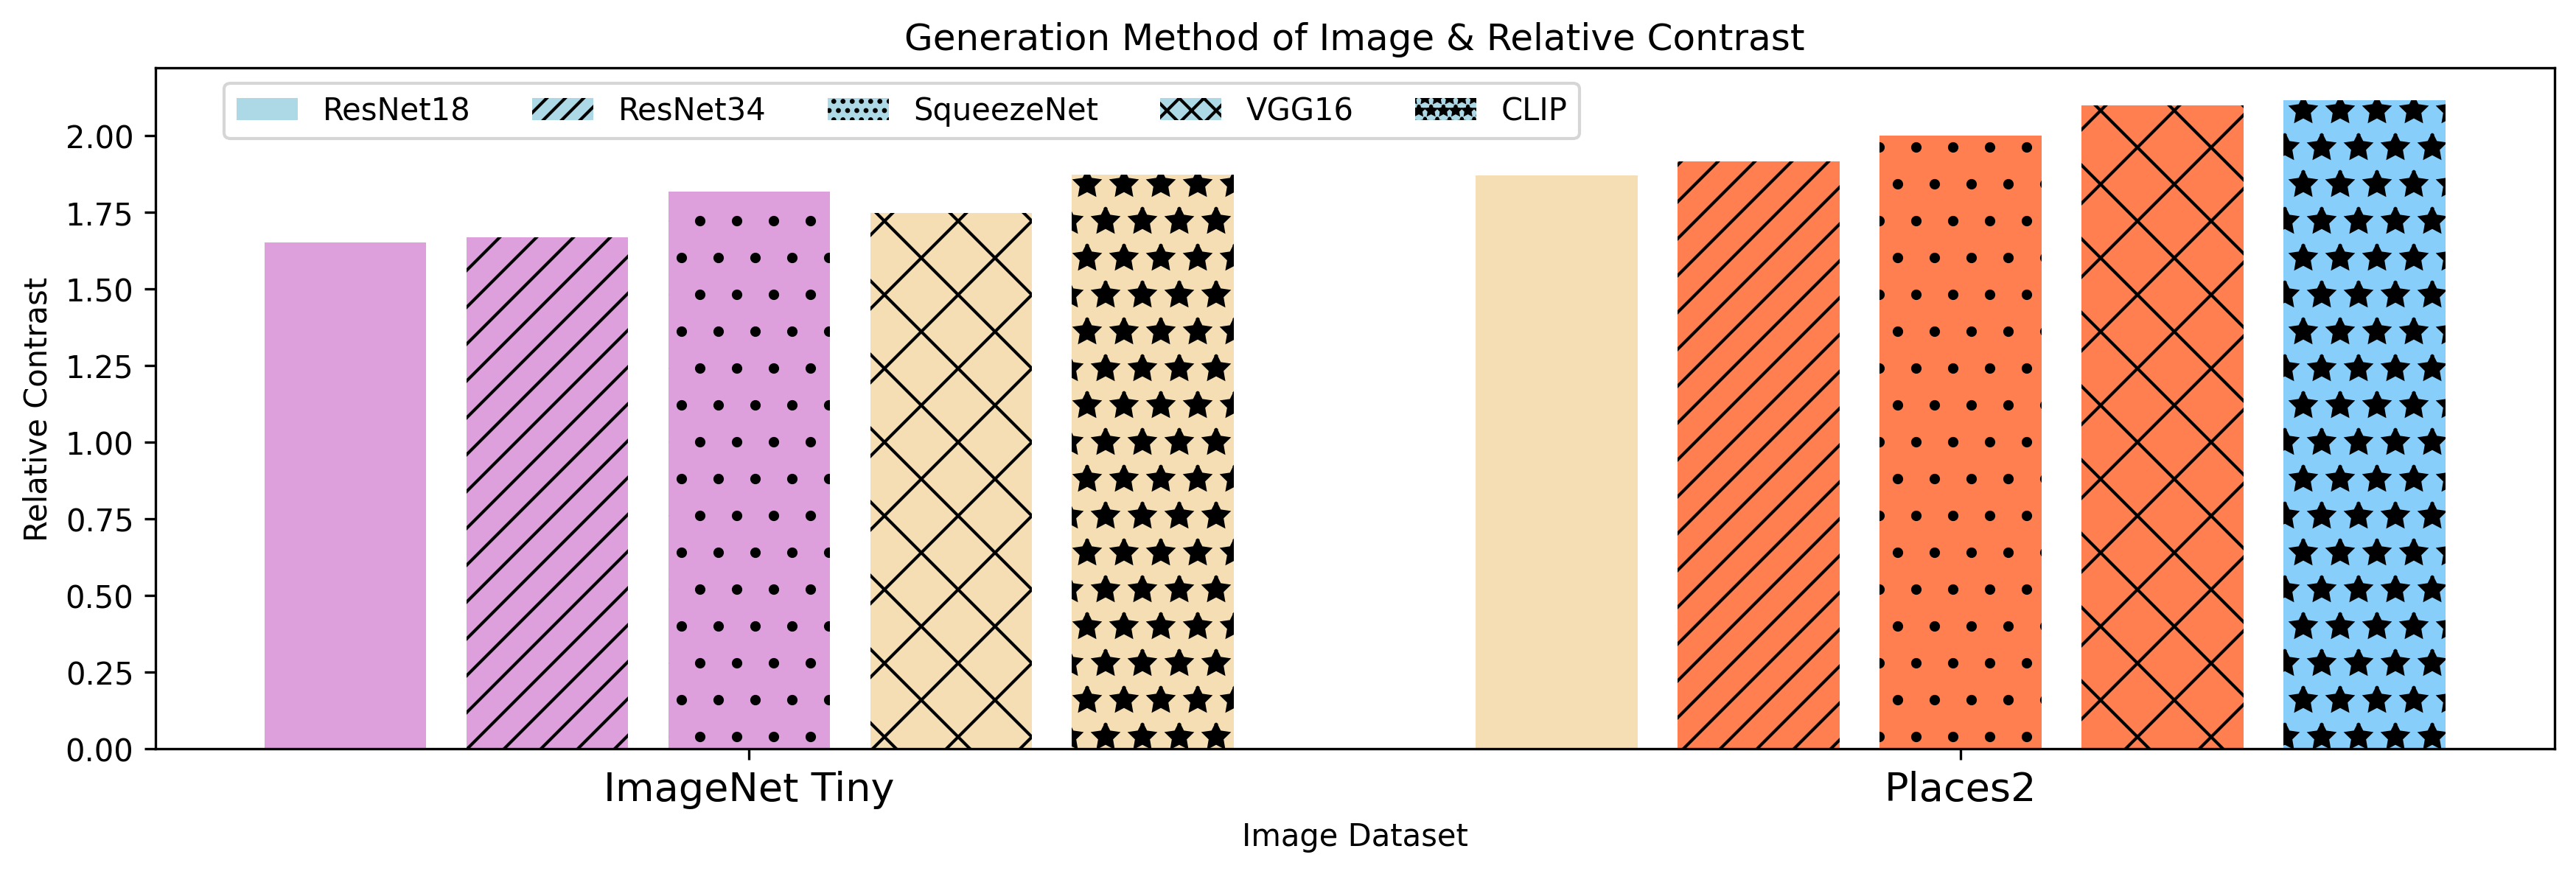}
    \caption{Explore the impact of generation method to the meaningfulness of NN search with image data}
    \label{fig:genmethod_image}
\end{figure}

Generally, with Figure: \ref{fig:genmethod_image}, it is obvious that the image datasets produce meaningful nearest neighbor search with dimensionality $512$, regardless of the generation method. More specifically, the image embedding generated by the CLIP model produces the most descent value of Relative Contrast.

In short, for image based vector / embedding at dimensionality of $512$, both of CNNs and CLIP model give meaningful and stable nearest neighbor search.

\subsection{Text Data}

For the text data, we conduct similar experiments studying how different generation method of text data could impact the meaningfulness of the NN search. Overall, three distinct generation methods of different era are used in this section. 

Specifically, the first one is the Latent Semantic Analysis (LSA) \cite{lsa}, which is a traditional yet classical method in Natural Language Processing (NLP). LSA aims to discover the hidden semantic relationship in large text corpus by reducing the dimensionality of word-document matrices with Singular Value Decomposition (SVD). The second one is Doc2Vec\cite{doc2vec}, which is one of the most prestigious non-transformer based embedding model with a foundation in Word2Vec\cite{word2vec}. Lastly, several transformer based text embedding models are used as the representative for the era of Large Language Model.

% Specifically, the first method is Latent Semantic Analysis (LSA), a traditional yet foundational technique in Natural Language Processing (NLP). LSA aims to uncover hidden semantic relationships within large text corpora by applying Singular Value Decomposition (SVD) to reduce the dimensionality of word-document matrices. The second method is Doc2Vec, a highly regarded non-transformer-based embedding model built on the principles of Word2Vec, known for effectively capturing contextual information at the paragraph level. Lastly, several transformer-based text embedding models represent the modern era of Large Language Models (LLMs), showcasing the power of deep learning and attention mechanisms for generating rich, nuanced text embeddings.

\begin{figure}[htp]
    \centering
    \includegraphics[width=\textwidth]{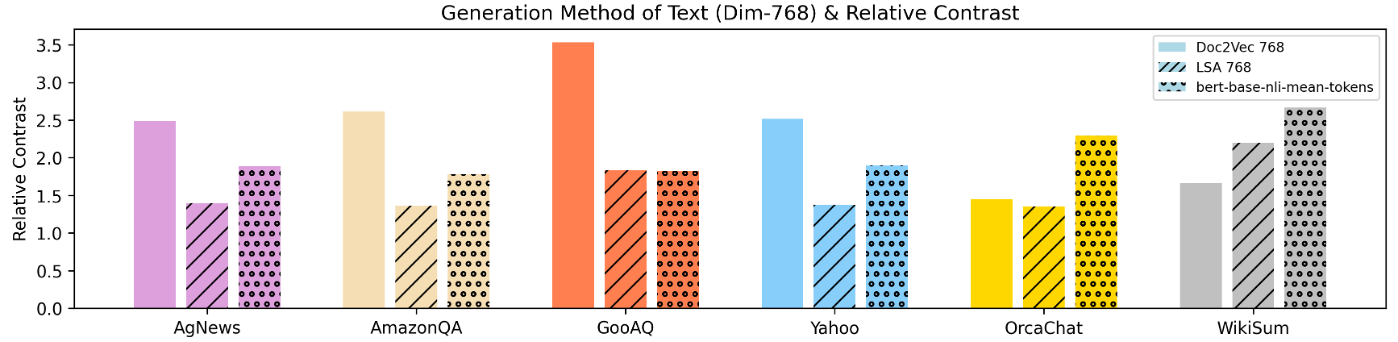}
    \includegraphics[width=\textwidth]{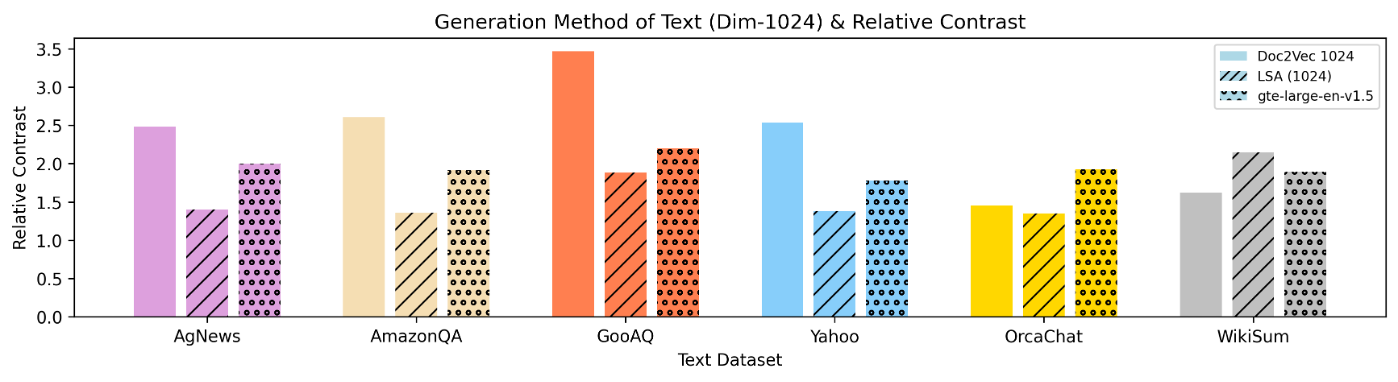}
    \caption{Explore the impact of generation method to the meaningfulness of NN search with text data (Upper: Dim768 || Lower: Dim1024)}
    \label{fig:genmethod_text}
\end{figure}

Technically, in this set of experiment, two embedding models of distinct dimensionality and architectures are utilized to improve the robustness of the experiments. Specifically, the encoder-only bert-base-nli-mean-tokens\cite{sentence-bert} with dimensionality of $768$ is used in the first set of experiment and the decoder-only gte-large-en-v1.5 \cite{gte-large} is used in the second set of experiment. In addition, as the typical manner for generating embedding using Doc2Vec is to train the dataset-specific model and then perform encoding, to ensure the fairness, identical training parameters are used among all of the datasets. 

According to Figure \ref{fig:genmethod_text}, it is easy to observe that both of Doc2Vec and transformer-based embedding models outperform the Latent Semantic Analysis in terms of the Relative Contrast, which demonstrates that these embedding models generally gives more meaningful NN search than LSA, given the same dimensionality. 

However, it is noticeable that, with some datasets, the transformer based embedding model produces a relatively lower Relative Contrast than the Doc2Vec; and the case is the opposite for the rest of datasets. One possible reason is as following. As the Doc2Vec model is trained per dataset, it is highly possible that the embedding gives meaningful Relative Contrast if the training parameters are optimized with respect to the dataset, otherwise, the performance degrades. On the contrary, as the transformer based embedding model is usually pre-trained on large text corpus, it will be much easier, faster, and more stable to use it to generate embedding than the Doc2Vec. But there is no denying that the Doc2Vec is still a performant model to generate text embedding for the purpose of Nearest Neighbor search.

\begin{figure}[htp]
    \centering
    \includegraphics[width=\textwidth]{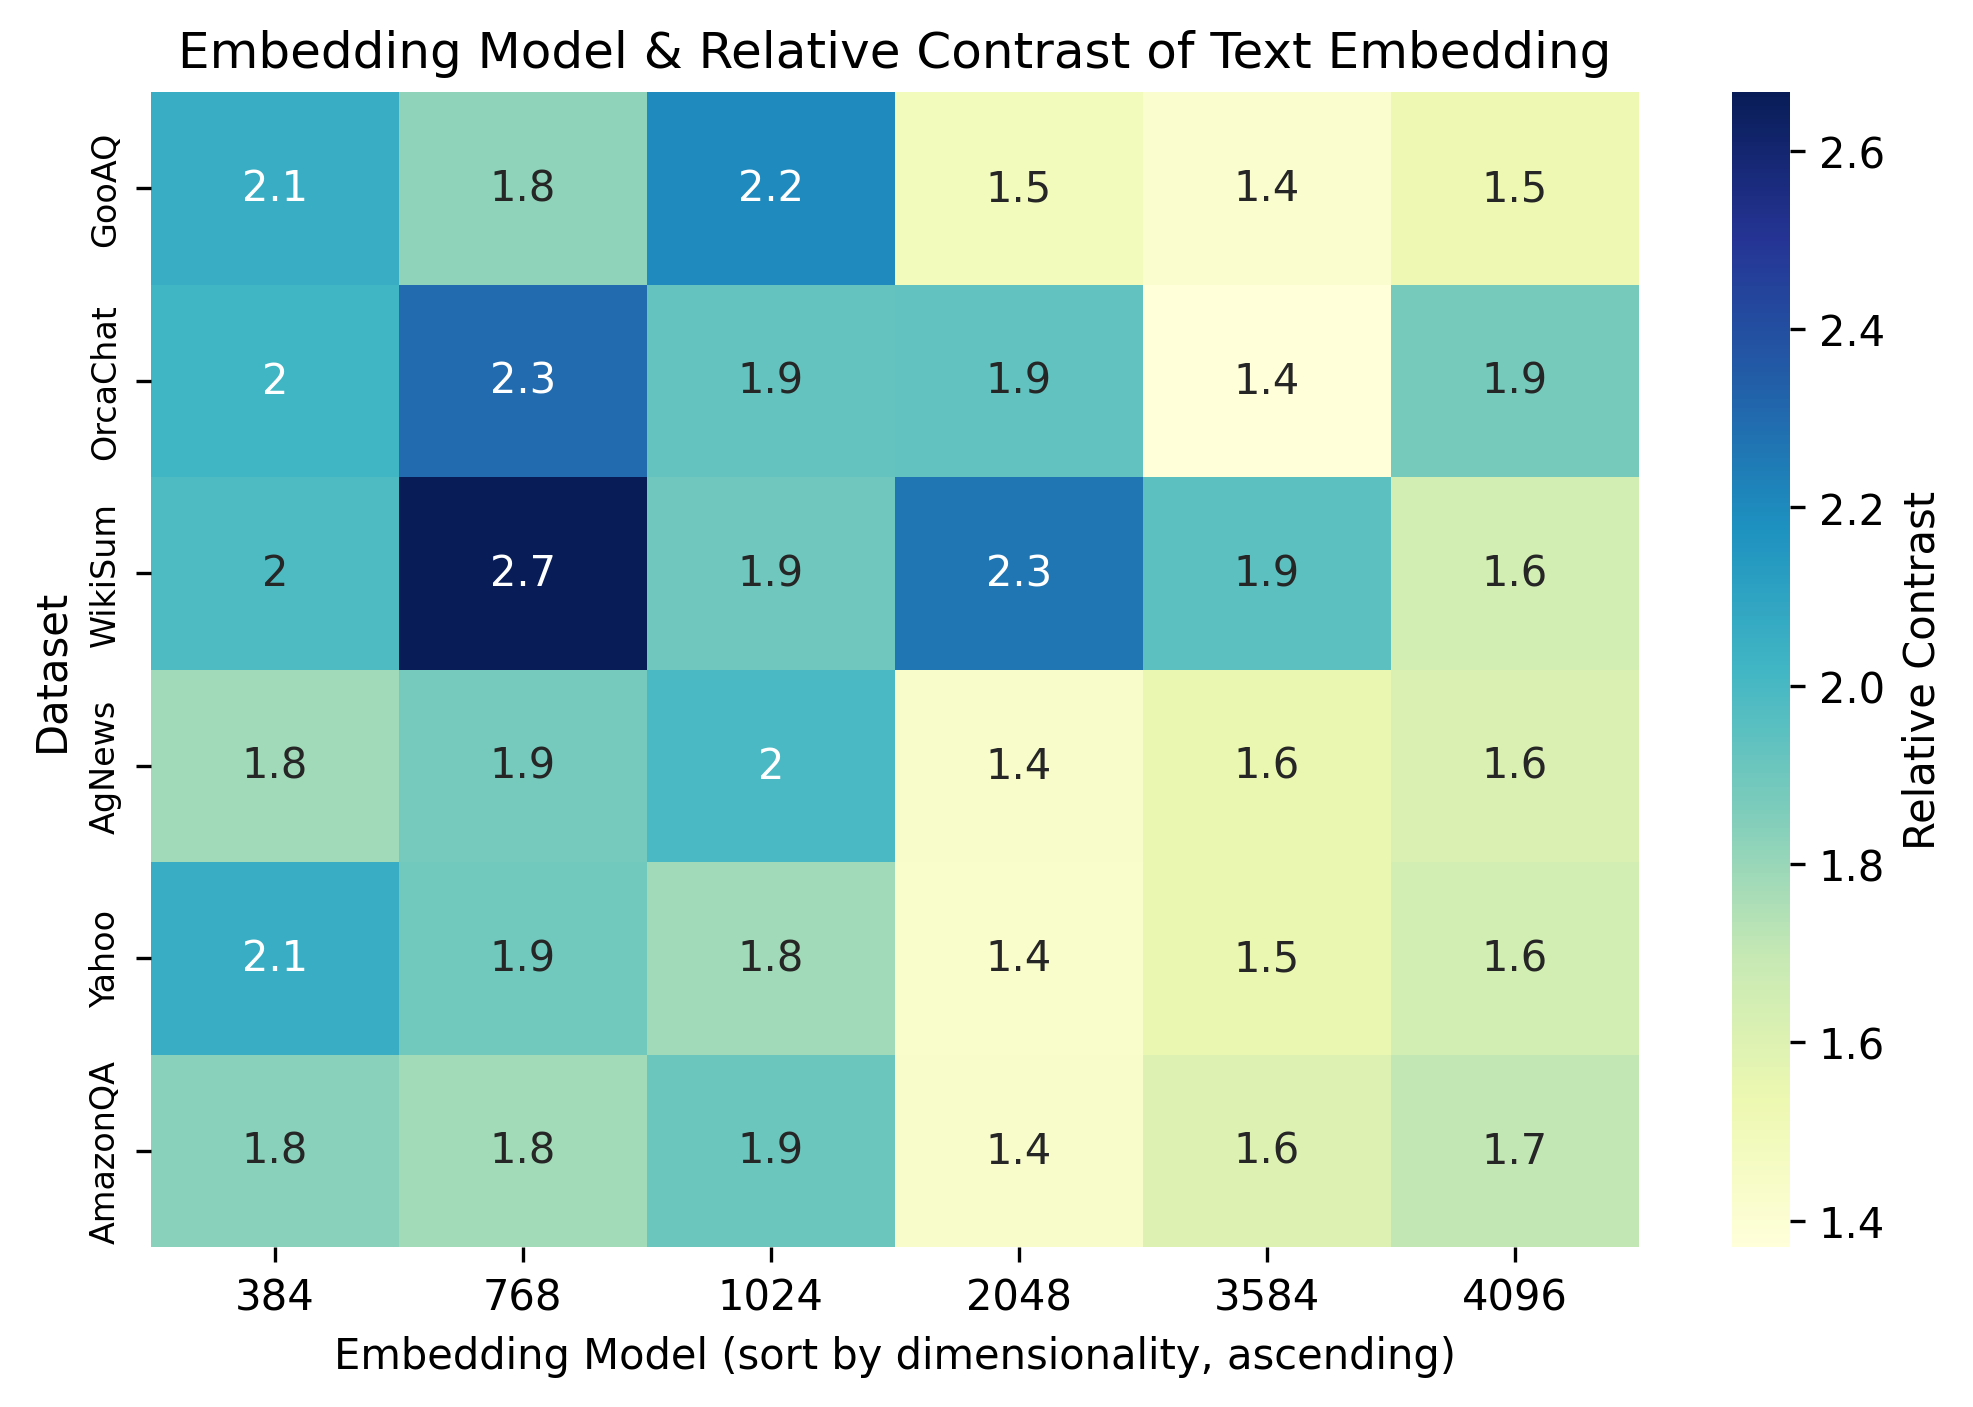}
    \caption{Relative Contrast \& Text with Different Embedding Model}
    \label{fig:vary_model}
\end{figure}

\section{Varying Embedding Models with Text Data}

In this experiment, we aim to provide an overview, on if using various types of embedding models will impact the meaningfulness of the nearest neighbor search in terms of the Relative Contrast. And each embedding model is represented by its corresponding dimensionality. Apart from the embedding models used in Table: \ref{tab:text_model}, we further extend the embedding models in Table: \ref{tab:text_model2}, where the diversity of the embedding model used in this study is substantially enhanced.

\begin{table}[!ht]
    \centering
    \small
    \begin{threeparttable}
        \begin{tabular}{|l|c|c|c|c|}
            \toprule
            \textbf{Model Name} & \textbf{Param} & \textbf{Max Input} & \textbf{Dim} & \textbf{Architecture} \\
            \midrule
            all-MiniLM-L6-V2 \cite{miniLM} & 22.7M & 256 & 384 & Encoder \\
            bert-base-nli-mean-tokens \cite{sentence-bert} & 109M & 512 & 768 & Encoder \\
            Alibaba-NLP/gte-large-en-v1.5 \cite{gte-large} & 434M & 8192 & 1024 & Encoder \\
            Wissam42/sentence-croissant-llm-base \cite{croissantllm} & 1280M & 2048 & 2048 & Decoder \\
            Alibaba-NLP/gte-Qwen2-7B-instruct \cite{gte-qwen} & 7.61B & 131072 & 3584 & Decoder \\
            nvidia/NV-Embed-v1 \cite{nvembed} & 7.85B & 32768 & 4096 & Decoder \\
            \bottomrule
        \end{tabular}
    \end{threeparttable}
    \caption{Comparison of different models.}
    \label{tab:text_model2}
\end{table}

With Figure: \ref{fig:vary_model}, we can easily infer that, for each dataset, different embedding models yield distinct Relative Contrast values, which completely complies with the common expectations. Generally, embeddings in lower-dimensional spaces ($384$, $768$, $1024$) tend to result in higher RC values, implying more meaningful NNS. Conversely, embeddings in higher-dimensional spaces ($2048$, $3584$, $4096$) typically exhibit lower RC values, a phenomenon likely attributed to the \textit{Curse of Dimensionality}. While there may be some impact from the embedding model, this impact is considered minor, as the models evaluated are among the best-performing according to the MTEB benchmark \cite{mteb-benchamrk}.

However, it is also noticeable that the relationship between dimensionality and RC is not completely predictable and linear, which fluctuates and always maintains the level of meaningful NN search.

\section{Generate Dataset of Text and Image Data}

\subsubsection{Components of Dataset}
Specifically, a complete dataset composes of two parts: the dataset and the query set. Different approaches are applied depending on the format of the original dataset. Specifically, for text datasets, if the raw dataset includes a predefined query set, it is be used directly as the query set. Otherwise, a specified number of points will be randomly sampled from the dataset to form the query set. For image datasets, where the original datasets typically include well-structured training, validation, and test set, the training set is used to generate the dataset, while the test set is used to create the query set. 

\subsubsection{Facilities}
All the embeddings are generated with a server with $\times 8$ NVIDIA A100 GPU Cards and $1.5$TB memory.
